# Supplementary material for: Self-Learning Monte Carlo Method
Source: arXiv:1610.03137 ancillary file (2016-12-20)
Supplement: Supplementary file 1 [file mlmcsm.pdf]

# Supplemental Material

Junwei Liu,[1] Yang Qi,[1] Zi Yang Meng,[2] and Liang Fu[1]

[1] *Department of physics, Massachusetts Institute of Technology, Cambridge, MA 02139, USA*

[2] *Institute of Physics, Chinese Academy of Sciences, Beijing 100190, China*

In this Supplemental Material, we provide reviews of previous works on the local and cluster update algorithms and technical details which are used in the main text.

## I. NUMERICAL ALGORITHMS

In this section, we provide technical details of the numerical algorithms used in our simulations. First, we briefly review the original Metropolis algorithm (the local update) and the Wolff algorithm (the cluster update). Then we present the details of the self-learning update, and the modified version where the cluster size is restricted.

All of the algorithms described in this section are realizations of the general Metropolis-Hastings algorithm [1]. In its most general form, an update in the Metropolis-Hastings algorithm contains two steps: First, starting from configuration $A$, a different configuration $B$ is constructed, with probability $Q(A \to B)$. The probability $Q(A \to B)$ takes different forms in update algorithms discussed below. Second, this update $A \to B$ is accepted by the probability $\alpha(A \to B)$ (often known as the acceptance ratio). Hence, the transition matrix element $p(A \to B)$ is given by $Q(A \to B)\alpha(A \to B)$. It is straightforward to verify that the following choice of $\alpha(A \to B)$ satisfies the detailed balance condition,

$$\alpha(A \to B) = \max\left\{1, \frac{W(B)}{W(A)}\frac{Q(B \to A)}{Q(A \to B)}\right\}. \tag{1}$$

### A. Local update

The most common update method, usually known as the local update, was first introduced in the original Metropolis algorithm [2]. When applied to the Ising model, the update algorithm randomly chooses a site, and flips the spin. Therefore, $Q(A \to B) = \frac{1}{N}$ if $B$ and $A$ differ by one spin flip, and zero if otherwise. Hence, we have $Q(A \to B) = Q(B \to A)$ for

any two configurations $A$ and $B$, and Eq. (1) gives the following acceptance ratio,

$$\alpha_L(A \to B) = \max\left\{1, \frac{W(B)}{W(A)}\right\}. \tag{2}$$

Since the local update only examines one spin at a time, configurations after one such trial are still strongly correlated. Therefore, following the convention in the literatures, we define one Markov-chain step as $N$ attempts of flipping a single spin, where $N$ is the number of sites. Hence, the computational complexity of one step is $O(N)$, which is the same as global updating algorithms, like the Wolff algorithm [3] will be discussed below. Therefore, this convention puts different algorithms on equal footing, as we compare their efficiency using their autocorrelation times.

### B. Wolff-cluster update

In each Markov chain step, the Wolff algorithm [3] constructs a cluster stochastically, and the resulting configuration B is obtained by flipping all spins in the cluster. Similar to other global update algorithms, the probability of constructing a certain cluster, $Q(A \to B)$, satisfies the condition that

$$\frac{Q(A \to B)}{Q(B \to A)} = \frac{W(B)}{W(A)}. \tag{3}$$

Thus, an ideal acceptance ratio $\alpha(A \to B) = 1$ satisfies the condition in Eq. (1). In other words, the Wolff update is always accepted.

The property of $Q(A \to B)$ in Eq. (3) is a result of how the cluster is constructed, which we now briefly review. The Wolff algorithm works for any two-body Ising models. Without losing generality, we demonstrate the algorithm using the nearest-neighbor Ising model,

$$H = -J \sum_{\langle ij \rangle} S_i S_j. \tag{4}$$

The algorithm of constructing a cluster can be summarized as follows,

1. Randomly select a site, flip the spin on it, and add it to the cluster $c$.

2. For each site $i$ in the cluster $c$, visit all links leading to its nearest neighbors which are not in the cluster already. Each link $\langle ij \rangle$ is activated with the probability

$$p(i \to j) = \min\{0, 1 - e^{2\beta J S_i S_j}\}. \tag{5}$$

3. If the link $\langle ij \rangle$ is activated, the site $j$ is added to the cluster, and the spin on it is flipped. The algorithm goes back to step 2.

4. The algorithm finishes when all links has been examined.

Now we consider the probability of constructing a cluster $c$ such that a configuration $A = \{S_i^A\}$ changes into configuration $B = \{S_i^B\}$, and compare it to the probability of constructing the same cluster $c$ such that B changes into A. The difference appears at the links on the boundary of $c$, which fail to activate in the process of constructing $c$. One can show that

$$\frac{Q(A \to B)}{Q(B \to A)} = \prod_{\langle ij \rangle, i \in c, j \notin c} \frac{1 - p(i \to j)_A}{1 - p(i \to j)_B} = \prod_{\langle ij \rangle, i \in c, j \notin c} e^{2\beta J S_i^B S_j^B} = \frac{W(B)}{W(A)}. \tag{6}$$

Thus, the probability $Q(A \to B)$ indeed satisfies the assertion in Eq. (3).

We notice that the computational complexity of Wolff algorithm is at most $O(N)$ per step, since the cluster size cannot exceed $N$.

### C. Self-learning update

As described in the main text, the SLMC algorithm uses an effective model to build a cluster with the Wolff algorithm, and tries to flip it according to the original Hamiltonian. Thus, the probability $Q(A \to B)$ is determined by the effective model,

$$\frac{Q(A \to B)}{Q(B \to A)} = \frac{W_{\text{eff}}(B)}{W_{\text{eff}}(A)}. \tag{7}$$

To satisfy the condition in Eq. (1), we need to use the following acceptance ratio,

$$\alpha(A \to B) = \max\left\{1, \frac{W(B)}{W(A)} \frac{W_{\text{eff}}(A)}{W_{\text{eff}}(B)}\right\}. \tag{8}$$

Using the relation $W = e^{-\beta E}$, we obtain the acceptance ratio

$$\alpha(A \to B) = \max\{1, e^{-\beta[(E_B - E_B^{\text{eff}}) - (E_A - E_A^{\text{eff}})]}\}, \tag{9}$$

which is the Eq. (3) of the main text.

### D. Restricted self-learning update

The Wolff algorithm can be generalized to include restrictions, often size limitations, on the growth of the cluster [4]. This is useful, for example, when big clusters have low acceptance ratios (like in our case), or when one wants to confine the cluster to a subset of the lattice to implement parallelism.

In the restricted Wolff algorithm, before trying to activate a link, the link is first tested to see if it violates a predetermined restriction. Links violates the restriction is logged during the process of constructing the cluster. This process can be viewed as a normal Wolff-cluster construction, on a model where all restriction-violating links are removed (i. e. $J$ is replaced by 0) from the nearest-neighbor Ising model. Hence, the probability $Q(A \to B)$ can be computed from this modified model,

$$\frac{Q(A \to B)}{Q(B \to A)} = \frac{W_{\text{eff}}(B)}{W_{\text{eff}}(A)} \prod_{\langle ij \rangle \in r} e^{-2\beta J S_i^B S_j^B}, \tag{10}$$

where the collection $r$ denotes the restriction-violating links logged during the construction of the cluster. Plugging this into Eq. (1), we get the following acceptance ratio,

$$\alpha(A \to B) = \max\left\{1, \frac{W(B)}{W(A)} \frac{W_{\text{eff}}(A)}{W_{\text{eff}}(B)} \prod_{\langle ij \rangle \in r} e^{2\beta J S_i^B S_j^B}\right\}. \tag{11}$$

In the Fig. 5 of main text, we present results of a restricted SLMC algorithm, where the growth of the cluster is limited to the area within $r = 40$ lattice spacing from the initial site (the Manhattan distance is used). Given this size limit, the cluster is constrained within a square-shape region, with an area $A_r = r^2/2$. Hence, in order to compare this algorithm on equal footing with the local and the unrestricted SLMC algorithms, we count $n = N/A_r$ cluster updates as one Monte Carlo step of restricted self-learning update (when $n$ is not an integer, we simply rescale the autocorrelation time by $n$.)

## II. PHASE DIAGRAM OF THE MODEL

To explore the phase diagram of the model in Eq. (1) of the main text, we compute the Binder cumulant (using the local update), for system sizes $L = 10, 20$ and 40. The result is shown in Fig. 1 The position of the crossing of the tree lines indicates that the transition happens at $T_c \simeq 2.493$.

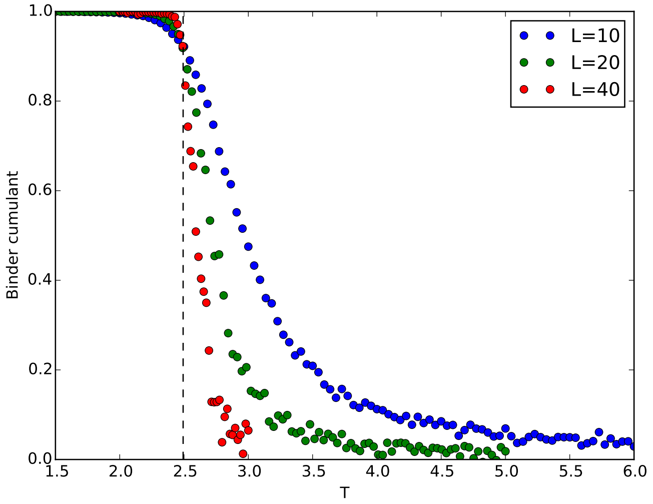


FIG. 1. The temperature dependence of the binder cumulant of the model in Eq. (1) of the main text. The bule, green and red dots represent systems with $L = 10, 20, 40$, respectively. The three lines at different system sizes cross approximately at one point, indicating $T_c = 2.493$.

## III. ITERATIVE FITTING OF THE EFFECTIVE MODEL

Here, we provide details of the iterative fitting process that produces the effective model. As explained in the main text, the effective model used in our SLMC algorithm is obtained from a sample of configurations, generated by Monte Carlo simulation with local update. But this approches is a dilemma by itself, i.e., we are developing the SLMC method to replace the inefficient local update, but it relies on the local update to provide an initial sample.

To solve this dilemma, we use an iterative learning process. We first run a simulation, at a temperature higher than the $T_c$, where the problem of critical slowdown is not severe, and the local update still works. We fit this first batch of data to the effective model, and obtain a parameter [$J_1^{\text{eff}}$ in Eq. (2) of the main text]. Using this parameter, we build an intermediate SLMC algorithm, and use it to generate a second sample. A more accurate effective model is then obtained by fitting the second batch of data to the effective model.

The SLMC method we present in the main text is produced with the following procedure: The model we consider ($J_1 = 1$ and $J_2 = 0.2$) has a critical temperature $T_c \simeq 2.493$. The first batch of data is generated at $T = 5$, using the local update. From the first iteration, we

obtain an effective model with $J_1^{\text{eff}} = 1.0726$. Using this effective model, the second batch of data is generated at $T_c$ with the SLMC. Finally an improved $J_1^{\text{eff}} = 1.1064$ is obtained using the second batch of data.

## IV. MEASURING THE AUTOCORRELATION FUNCTION

The correlation between configurations in a Markov chain can be gauged by the autocorrelation function. We consider a Markov chain $\cdots \to A(t-1) \to A(t) \to A(t+1) \to \cdots$, where $t$ labels the steps of the chain, and $A(t)$ denotes the configuration at step $t$. Here, we choose the letter $t$, since it can be viewed as the time variable, i.e., Monte Carlo time of the Markov chain. Furthermore, we consider a particular observable $O = O[A]$ (like the order parameter or the energy), and the values of the observable for configurations of the Markov chain forms a time sequence,

$$\cdots \to O(t-1) \to O(t) \to O(t+1) \to \cdots , \quad O(t) = O[A(t)]. \tag{12}$$

An autocorrelation function can be defined for this time sequence,

$$\mathcal{A}_O(\Delta t) = \langle O(t)O(t+\Delta t)\rangle - \langle O(t)\rangle^2, \tag{13}$$

where the average $\langle\cdot\rangle$ is taken on the time sequence.

If the Markov chain is not correlated, which is the ideal case, the autocorrelation function defined in Eq. (13) should decay exponentially,

$$\mathcal{A}_O(\Delta t) = \mathcal{A}_0 e^{-\Delta t/\tau}, \tag{14}$$

and the decay-time constant $\tau$ is called the autocorrelation time.

We measure the autocorrelation function $\mathcal{A}_O(\Delta t)$ in the following way. After an initial process during which the Markov chain converges to its stable distribution, a total number of $\mathcal{N}$ measurements $O(t)$ are drawn from $\mathcal{N}$ Markov-chain steps. For any $\Delta t$, the autocorrelation function is given by the average over the following $\mathcal{N} - \Delta t$ samples,

$$\mathcal{A}_O(\Delta t) = \frac{1}{\mathcal{N} - \Delta t} \sum_{t=0}^{\mathcal{N}-\Delta t} O(t)O(t+\Delta t) - \left[\frac{1}{\mathcal{N}} \sum_{t=0}^{\mathcal{N}} O(t)\right]^2 . \tag{15}$$

[1] W. K. Hastings, Biometrika **57**, 97 (1970).

[2] N. Metropolis, A. W. Rosenbluth, M. N. Rosenbluth, A. H. Teller, and E. Teller, J. Chem. Phys. **21**, 1087 (1953).

[3] U. Wolff, Phys. Rev. Lett. **62**, 361 (1989).

[4] G. T. Barkema and J. F. Marko, Phys. Rev. Lett. **71**, 2070 (1993).
